# Supplementary material for: Blind-Match: Efficient Homomorphic Encryption-Based 1:N Matching for Privacy-Preserving Biometric Identification
Source: arXiv:2408.06167 source file (2024-10-13)
Supplement: Supplementary file 1 [file Appendix.tex]

\onecolumn
\section{Optimized HE-Cossim Algorithm}
\label{sec:A:}

\subsection{Conjugate Invariant Ring Setting}
\label{secsec:Conjugate_Invariant_Ring_setting}
\sysname uses the CKKS scheme which is based on the RLWE over Conjugate-invariant Ring, which is a subring of a cyclotomic ring. The conjugate Invariant Ring supports twice as many real numbers in encryption, it reduces the wasted slots of imaginary parts in the arithmetic operation. The CKKS scheme based on the RLWE problem in the Conjugate Invariant Ring has the same security level as that of the general CKKS scheme~\cite{kim2019approximate}.

\subsection{Operations of HE}
\label{subsec:operations_of_he}
$Add$, $Mul$, $Rot$, and $Res$ are basic operation in CKKS scheme. Let $N$ is the \textit{number of slots} and $\mathbf{v_1}, \mathbf{v_2}$ are two real vectors with size $N$. $C(\mathbf{v_1}), C(\mathbf{v_2})$ denotes ciphertexts of $\mathbf{v_1}, \mathbf{v_2}$ each other. Then, each operations are defines as follows:
\begin{itemize}[noitemsep]
    \item Add (P): $Add(C(\mathbf{v_1}), \mathbf{v_2}) = C(\mathbf{v_1} \oplus \mathbf{v_2})$ 
    \item Add (C): $Add(C(\mathbf{v_1}), C(\mathbf{v_2})) = C(\mathbf{v_1} \oplus \mathbf{v_2})$ 
    \item Mul (P): $Mul(C(\mathbf{v_1}), \mathbf{v_2}) = C(\mathbf{v_1} \otimes \mathbf{v_2})$ 
    \item Mul (C): $Mul(C(\mathbf{v_1}), C(\mathbf{v_2})) = C(\mathbf{v_1} \otimes \mathbf{v_2})$ 
    \item Rot : $Rot(C(\mathbf{v}), r) = C(v_{r}, v_{r+1}, ... , v_{N-1}, v_{1}, ... , v_{r-1})$ \\
    where $\mathbf{v} = (v_{1}, v_{2}, ..., v_{N})$ and $r$ is a non-zero integer.
\end{itemize}

(P) means that the operation is defined on between a ciphertext and a plaintext (or a constant).  (C) means that the operation is defined between two ciphertexts. The notation $\oplus, \otimes$ means that the element-wise addition and multiplication respectively. In this paper, we only use the $Add(C)$ in addition, we simply denote $Add$ instead of $Add(C)$. The ciphertext in the CKKS scheme contains two elements, but after the multiplication, the number of elements grew to three. Thus, the re-linearization operation is needed to reduce the three elements as two elements of the output ciphertext of multiplication. The notation $Mul$ means the multiplication with re-linearization. $Res$ is the rescale operation, which reduces the noise that is increased after multiplication. $Res$ keeps the precision of the ciphertext, however the level $l$ is decreased to $l-1$ after $Rel$ operation is conducted.

\subsection{\textit{HE-Cossim Algorithm}}
\label{secsec:he_cossim_algorithm}
Algorithm~\ref{alg:he_based_cosine_similarity} describes the mechanism of the \textit{HE-Cossim}. The algorithm is used in the SoTA HE-based privacy-preserving biometric identification research~\cite{ibarrondo2023grote}.
\begin{algorithm}[!ht]
   \caption{\textit{Conventional HE-Cossim}}
   \label{alg:he_based_cosine_similarity}
\begin{algorithmic}[1]
   \STATE {\bfseries Input:} $C_{u}, C_{s}$, $fv_{s}$
   \STATE {\bfseries Output:} $C_{out}$
   \STATE $C_{out} := Rescale(Mul(C_{u}, C_{s}))$
   \FOR{$i=1$ {\bfseries to} $\log{fv_{s}}$} 
   \STATE $C_{out} = Add(Rot(C_{out}, 2^{i-1}), C_{out})$
   \ENDFOR
\end{algorithmic}
\end{algorithm}

\subsection{Proof of Theorem~\ref{thm:1}}
\label{secsec:proof_of_thm1}
Remind that $N, l$ are \textit{number of slots}, and \textit{level}. $R$=$N/4$ is the total number of subjects used in the identification. We proved two statements: uniquely existence of the $X$, and the correctness of the range of $X$.
For the convenience of the proof, let's assume that X has a real number range as its domain.

\begin{proof}
Using Proposition~\ref{prop:2}, Proposition~\ref{prop:3}, and Proposition~\ref{prop:4}, the total identification time of \sysname can be expressed as a function of $X$ where $X$ is the number of ciphertexts used in Algorithm~\ref{alg:input_ctxt_expansion_methods}. Unlike the original statements in Proposition~\ref{prop:2}, Proposition~\ref{prop:3}, the level $l$ is decreased because of the rescale operation $Res$. Denote that $F(X)$ is the total identification time function of \sysname.
Then, $F(X)$ can be written as the form: \\
\begin{align*}
   F(X) &= \underset{\text{by Proposition~\ref{prop:3}}}{\underline{\textit{X} \cdot ((T_{Mul(P),l} + T_{Res,l}) + \log{X} \cdot (T_{Res, l-1}+T_{Mul(C),l-1}))}} \\
  &+ \underset{\text{by Proposition~\ref{prop:2}}}{\underline{\left\lceil \left(\frac{fv_{s}^{\prime}}{X}\right) \right\rceil \cdot  (X \cdot(T_{Mul(C), l-1}+T_{Res,l-1} + T_{Add, l-2}) + (\log{fv_{s}^{\prime}}-\log{X})\cdot(T_{Rot, l-2}+T_{Add, l-2})}})\\
  &+ \underset{\text{by Proposition~\ref{prop:4}}}{\underline{\left\lceil \left(\frac{fv_{s}^{\prime}}{X}\right) \right\rceil \cdot (\log{fv_{s}^{\prime}}-\log{X}) \cdot(T_{Mul(P),l-2}+T_{Rot, l-2}+T_{Add, l-2})}} \\
\end{align*}

Remind that $N$=$8,192$, $l$=$3$, and $R$ = $2,048$. Then by Table \ref{table:operation_time_with_l}, $T_{Mul(P), 3}= 1.25, T_{Res,3}=1.30, T_{Res,2}=0.95, T_{Mul(C),2}=5.49, T_{Mul(P),1}=0.76, T_{Rot,1}=2.95, T_{Add,1}=0.09$ . Then, the above equation can be written as follows:

\begin{align*}
   F(X) &= X \cdot ((1.25 + 1.30) + \log{X} \cdot (0.95 +5.49)) \\
  &+ \left\lceil \left(\frac{fv_{s}^{\prime}}{X}\right) \right\rceil \cdot  (X \cdot(5.49+0.95 + 0.09) + (\log{fv_{s}^{\prime}}-\log{X})\cdot(2.95+0.09))\\
  &+ \left\lceil \left(\frac{fv_{s}^{\prime}}{X}\right) \right\rceil \cdot (\log{fv_{s}^{\prime}}-\log{X}) \cdot(0.76+2.95+0.09) \\
  &= 2.55X + 6.44X\log{X} + 6.53fv_{s}^{\prime} + \frac{6.84fv_{s}^{\prime}}{X} \cdot (\log{fv_{s}^{\prime}} - \log{X})\\
\end{align*}
% \begin{align*}
%    &F(X) = \underset{\text{by Proposition~\ref{prop:3}}}{\underline{\textit{X} \cdot ((T_{Mul(P),l} + T_{Res,l}) + \textit{log{X}} \cdot (T_{Res, l-1}+T_{Mul(C),l-1}))}} \\
%   &+ \quad \underset{\text{by Proposition~\ref{prop:2}}}{\underline{\lceil (fv_{s} \cdot R) / (N \cdot X) \rceil \cdot  (X \cdot(T_{Mul(C), l-1}+T_{Res,l-1} + T_{Add, l-2}) + (log{fv_{s}}-log{X})\cdot(T_{Rot, l-2}+T_{Add, l-2})}})\\
%   &+ \quad \underset{\text{by Proposition~\ref{prop:4}}}{\underline{\lceil (fv_{s} \cdot R) / (N \cdot X) \rceil \cdot (log{fv_{s}}-log{X}) \cdot(T_{Mul(P),l-2}+T_{Rot, l-2}+T_{Add, l-2})}} \\
% \end{align*} 
% Remind that $N$=$8,192$, $l$=$3$, and $R$ = $2,048$. Then by Table \ref{table:operation_time_with_l}, $T_{Res,3}=0.312 , T_{Mul(P), 3} = 0.325, T_{Res,2}=0.229, T_{Mul,2}=1.508, T_{Mul,1}=0.842, T_{Rot,1}=0.783, T_{Add,1}=0.026$. Then, the above equation can be written as follows: 
% \begin{align*}
%    &F(X) = \textit{X} \cdot ((1.249 + 1.295) + \textit{log X} \cdot (0.953 +5.487)) \\
%   &+ \quad \lceil (fv_{s} \cdot 2,048) / (8,192 \cdot X) \rceil \cdot  (X \cdot(5.487+0.953 + 0.087) + (log{fv_{s}}-log{X})\cdot(2.954+0.087))\\
%   &+ \quad \lceil (fv_{s} \cdot 2,048) / (8,192 \cdot X) \rceil \cdot (log{fv_{s}}-log{X}) \cdot(0.764+2.954+0.087) \\
%   &= \quad  X \cdot 2.544 + X \cdot \textit{log X}  \cdot 6.44 + (fv_{s}/ 4)\cdot (1/X) \cdot (X \cdot 6.527 + (\log fv_s - \textit{log X}) \cdot 6.846)\\
% \end{align*}  

\textbf{Uniquely Existence of the number of input ciphertext.}\\
 Differentiate the above function with respect to $X$, then \\
\begin{align*}
F^{\prime}(X) &= 2.55 + 6.44\left(\log{X} + \frac{1}{\ln{2}}\right) - \frac{6.84fv_{s}^{\prime}}{X^2} \left(\log{fv_{s}^{\prime}} - \log{X} + \frac{1}{\ln{2}}\right) \\
&\approx 11.88 + 6.44\log{X} - \frac{6.84fv_{s}^{\prime}}{X^2} \left(\log{fv_s^{\prime}} - \log{X} + 0.69\right)
\end{align*}
For all $fv_s^{\prime} \geq 4$,
\begin{align*}
F^{\prime}\left({fv_{s}^{\prime}}^{1/3}\right) &= 11.88 + 2.15 \log{fv_{s}^{\prime}} - 6.84 {fv_{s}^{\prime}}^{1/3} \cdot \left(\frac{2}{3}\log{fv_{s}^{\prime}} + 0.69\right) \\
&= 11.88 - 4.72 {fv_{s}^{\prime}}^{1/3} + \left(2.15 - 4.56 {fv_{s}^{\prime}}^{1/3}\right) \cdot \log{fv_{s}^{\prime}} \\
&< 0 \\
\end{align*}
For all $fv_s^{\prime} \leq 2^{32}$,
\begin{align*}
F^{\prime}\left(fv_{s}^{1/2}\right) &= 11.88 + 3.22 \log{fv_{s}^{\prime}} - 6.84 \left(\frac{1}{2} \log{fv_{s}^{\prime}} + 0.69\right) \\
&= 7.16 - 0.20 \log{fv_{s}^{\prime}}\\
&> 0
\end{align*}
For all $X \in \left(1, fv_s^{\prime}\right)$,
\begin{align*}
F^{\prime \prime}(X) &= \frac{6.44}{X \ln{2}} + \frac{13.68 fv_{s}}{X^{3}} \left(\log{fv_{s}^{\prime}} - \log{X} + 0.69\right) + \frac{fv_s^{\prime} \cdot \frac{6.84}{\ln{2}}}{X^{3}} \\
&\approx \frac{9.29}{X} + \frac{fv_s^{\prime}}{X^3} \cdot \left(13.68 \log{\left(\frac{fv_s^{\prime}}{X}\right)} + 9.87 fv_s^{\prime} + 9.44 \right) \\
&> 0 \\
% &= \quad 6.44/X + \cdot (3.423 \cdot fv_{s}) \cdot (\log{fv_s^{\prime}} - \log X + 0.5) / X^{3} \\
\end{align*}

The second derivative $F^{\prime \prime}$ is positive in the domain $\left(1, fv_s^{\prime}\right)$, the derivative $F^{\prime}$ is a continuous function and a strictly increasing function. 
% In this paper, as we specifically consider the case where $X$ is a natural number. 
Our goal is to demonstrate that there uniquely exists $X$ within the interval $\left({fv_{s}^{\prime}}^{1/3}, {fv_{s}^{\prime}}^{1/2}\right)$ 
% if ${fv_{s}^{\prime}} \leq 2^7$
that makes the total identification time to minimize.

% Please note that the total authentication time has same value to continuous function F(X) in $\mathbb{N}$, is discrete in $\mathbb{N}$.
\textbf{Existence.}\\
For the convenience of the proof, let's assume $a={fv_{s}^{\prime}}^{1/3}$ and $b={fv_{s}^{\prime}}^{1/2}$. Note that $F^{\prime}(a) < 0$ and $F^{\prime}(b) > 0$. By Intermediate Value Theorem, there is an $c \in (a, b)$ such that $F^{\prime}(c)=0$. Since $F^{\prime \prime}(c)>0$, $F(c)$ is a local minimum.

\textbf{Uniqueness.} \\ 
Suppose that there are two local minimum values $c_1, c_2 \in (a, b)$ such that $F^{\prime}(c_1)=F^{\prime}(c_2)=0$. By Rolle's theorem, there is a $c_3 \in (c_1, c_2)$ such that $F^{\prime \prime}(c_3)=0$. This presents a contradiction as $F^{\prime \prime}$ is positive in the domain $(1, fv_s^{\prime})$. Therefore, the local minimum is unique.

Thus, $F$ has a unique minimum in the range $\left({fv_s^{\prime}}^{1/3}, {fv_s^{\prime}}^{1/2}\right)$.

\end{proof}

\onecolumn
\section{Execution Times of \sysname}
\label{sec:b_experiments}
Table~\ref{table:experim_results_about_T_128_extension} is the extension of Table~\ref{table:experim_results_about_T_128} added the operation times of $N_{in}=32$.

\begin{table}[ht]
\caption{The results on the total identification time ($ms $) according to the number of input ciphertexts. The 6,144 face images (from the IJB-C dataset) are used for evaluation. The used parameter setting are $N$=$8,192$, $l=3$, and feature vector size is $128$.}
\vspace{0.26cm}
\centering\resizebox{0.7\linewidth}{!}{

\begin{tabular}{c|c|c|c|c|c}
\noalign{\smallskip}\noalign{\smallskip}
\toprule[1.3pt]
\textit{op} \textbackslash $N_{in}$ & 2 & 4 & 8 & 16 & 32\\
\hline
\hline
Enc & \multicolumn{5}{c}{29.58 (4.32)} \\
\hline
Dec & \multicolumn{5}{c}{24.35 (1.57)} \\
\hline
Infer & \multicolumn{5}{c}{129.23 (8.24)}  \\
\hline
Matching & 650.92 (13.38) & 451.66 (9.27)& 457.02 (13.92) & 652.14 (13.45) & 1221.276 (25.11)\\
\hline
Network & 108.52 (7.39) & 102.60 (12.71) & 100.03 (12.50) & 105.55 (19.93) & 107.337 (14.35)\\
\hline
Total & 942.59 (18.59) & 737.41 (13.49) & 740.202 (12.72) & 940.84 (12.73) &  1551.77 (25.05)\\
\bottomrule
\end{tabular}}
\label{table:experim_results_about_T_128_extension}
\end{table}

The total time of $N_{in}=32$ is almost two times that of $N_{in}=8$. The result shows that the selection of best $N_{in}$ makes incredible performance improvements. The result of \sysname's execution time on $fv_{s} = 64$ is described in Table~\ref{table:experim_results_about_T_64}. 

\begin{table}[!ht]
\caption{The results on the total identification time ($ms $) according to the number of input ciphertexts. The 6,144 face images from the IJB-C dataset are used for evaluation. The used parameter settings are $N=8,192$, $l=3$, and the feature vector size is $64$.}
\vspace{0.26cm}
\centering\resizebox{0.7\linewidth}{!}{
\setlength{\tabcolsep}{10pt}

\begin{tabular}{c|c|c|c|c}
\noalign{\smallskip}\noalign{\smallskip}
\toprule[1.3pt]
\textit{op} \textbackslash $N_{in}$ & 2 & 4 & 8 & 16\\
\hline
\hline
Enc & \multicolumn{4}{c}{29.58 (4.32)} \\
\hline
Dec & \multicolumn{4}{c}{24.35 (1.57)} \\
\hline
Infer & \multicolumn{4}{c}{129.23 (8.24))} \\
\hline
Matching & 318.07 (10.47) & 262.18 (6.41) & 318.90 (6.46) & 537.87 (13.61)  \\
\hline
Network & 88.29 (11.182) & 92.61 (22.05) & 92.18 (23.88) & 90.96 (20.20)\\
\hline
Total & 589.51 (8.62) & 537.94 (18.65) & 594.33 (18.73) & 811.99 (15.96) \\
% \hline
\bottomrule
\end{tabular}}
\label{table:experim_results_about_T_64}
\end{table}

When $N_{in} = 4$, the matching time and total time are minimal. Since 4 is nearest in the interval ($4=64^{1/3}, 8=64^{1/2}$) (in this case, 8 is also the nearest value of the interval), the result also gives a justification of Theorem~\ref{thm:1}.

\onecolumn
\section{Fingerprint Datasets and Effects of Preprocessing}
\label{sec:c_experiments}

\subsection{Dataset Description}
\label{subsec:dataset_description}

\begin{table}[!ht]
\caption{Summary of fingerprint datasets for identification/authentication systems. Especially PolyU and CASIA datasets are publicly available. The subsets of PolyU share the same IDs however, the subsets of FVC differ from each other. The number of volunteers of FVC 2000 DB2 was not reported.}
\centering\resizebox{\linewidth}{!}{

\begin{tabular}{lcccccccc}
\noalign{\smallskip}\noalign{\smallskip}
\toprule[1.3pt]
\textbf{Datasets} & \textbf{\# Participants} & \textbf{\# Subjects }& \textbf{\# Images} & \textbf{Scale} & \textbf{Openness} &\textbf{Scan} & \textbf{Finger}& \textbf{Section}\\
\hline
\hline
PolyU (Processed) Contactless&\multirow{2}{*}{300}&\multirow{2}{*}{496}&\multirow{2}{*}{ 2,976}&350x255&\multirow{2}{*}{Restricted public} &Contactless&\multirow{2}{*}{N/A} &\multirow{2}{*}{~\ref{subsec:performance}~\&~\ref{subsubsec:polyu_dataset}}\\
PolyU Contact-based& && &328x356 & &Contact&&\\
% PolyU Contactness & 300 & 496 & 2,976 & 328x356 & Restricted public & Touch & N/A& \checkmark\\
\hline
% FVC 2000 DB1 & - & 110 & 880 & 300x300 & Public & Contact &Index\&Middle&-\\
FVC 2000 DB2 & - & 110 & 880 & 256$\times$364 & Public & Contact &Index\&Middle&~\ref{subsubsec:fvc_dataset}\\
% FVC 2000 DB3 & 19 & 110 & 880 & 448x478 & Public & Contact &Thumb\&Index\&Middle&-\\
FVC 2000 DB4 & N/A & 110 & 880 & 240$\times$320 & Public & Synthesized&N/A & ~\ref{subsubsec:fvc_dataset}  \\
FVC 2002 DB1 & 30 & 110 & 880 & 388$\times$374 & Public & Contact &Index\&Middle &~\ref{subsec:ablation_study}~\&~\ref{subsubsec:fvc_dataset}\\
% FVC 2002 DB2 & 30 & 110 & 880 & 296x560 & Public & Contact &Index\&Middle& -\\
FVC 2002 DB3 & 30 & 110 & 880 & 640$\times$480 & Public & Capacitive &Index\&Middle&~\ref{subsubsec:fvc_dataset}\\
FVC 2002 DB4 & N/A  & 110 & 880 & 268$\times$384 & Public & Synthesized & N/A &~\ref{subsubsec:fvc_dataset}\\
FVC 2004 DB1 & 30 & 110 & 880 & 328$\times$364 & Public & Contactless &Index\&Middle &~\ref{subsubsec:fvc_dataset}\\
% FVC 2004 DB2 &30& 110 & 880 & 300x480&Public &Contactless&Index\&Middle& \checkmark\\
% FVC 2004 DB3 & 30 & 110 & 880 & 288x384 & Public & Thermal &Index\&Middle& - \\
FVC 2004 DB4 & N/A & 110 & 880 & 288$\times$284 & Public & Synthesized& N/A &~\ref{subsubsec:fvc_dataset} \\
\hline
CASIA fingerprint v5 & 500 & 4,000 & 20,000 & 328$\times$356 & Public& Rotated & Thumb\&Index\&Middle\&Ring&~\ref{subsubsec:casia_dataset}  \\
\toprule[1.3pt]
\end{tabular}}
\label{table:summary_datasets}
\end{table}

Table~\ref{table:summary_datasets} summarizes the fingerprint datasets used in our experiments. We choose the publicly opened fingerprint datasets that are collected using various scan methods to prove the generality of the experiment. The number of subjects in each FVC fingerprint dataset is relatively small to face datasets for identification experiments, we use the combined FVC2000 DB2, DB4, FVC2002 DB1, DB3, DB4, and FVC2004 DB2, DB4. The detailed usage of fingerprints in this paper is denoted in \textbf{Section} field in Table~\ref{table:summary_datasets}.

\begin{figure}[ht]
\vskip 0.2in
% \begin{center}
\centerline{\includegraphics[width=\columnwidth]{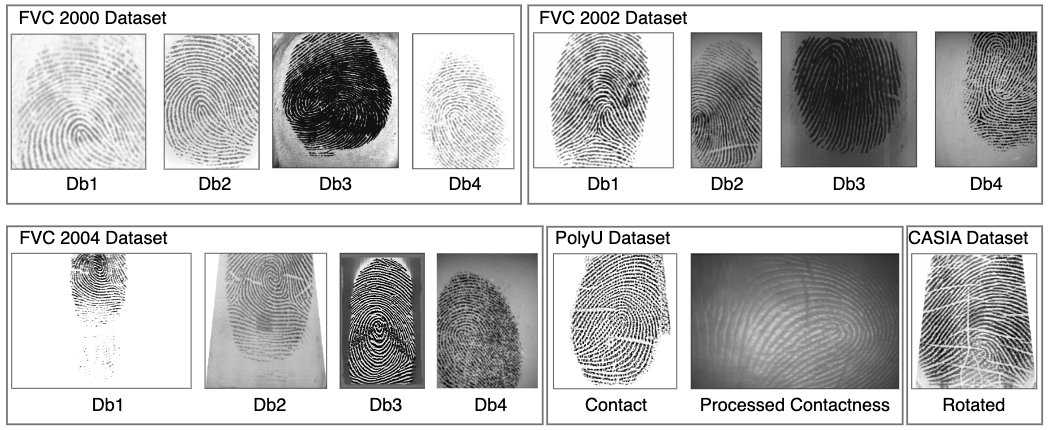}}
\caption{Samples of fingerprint datasets used in experiments.}
\label{fig:various_fingerprint_images}
% \end{center}
\vskip -0.2in
\end{figure}

\subsubsection{PolyU Dataset}
\label{subsubsec:polyu_dataset}
The PolyU Cross Sensor dataset~\cite{lin2018matching} contains contact-based and contactless-2D fingerprint images. It consists of a two-session cross-sensor fingerprint dataset. Each subject has 6 fingerprint images and the first session consists of 336 subjects and the second session consists of 160 subjects. The contact-based images are gray-scale with 328$\times$356-pixel resolution. For the contactless-2D images, they provide original high-resolution images with 1400$\times$900 and processed contactless-2D fingerprint images with 350$\times$225-pixel resolution. The processed one is cut the redundant non-fingerprint pattern area off. We utilized contact-based and processed contactless PolyU datasets for our experiments. Since Blind-Touch only shows the authentication performance on processed contactless PolyU dataset, we benchmark \sysname against Blind-Touch using processed contactless images. (See~\ref{subsec:performance} and Table~\ref{table:score_of_polyU_dataset}) Some samples of this dataset are in Figure~\ref{fig:various_fingerprint_images} and the summarized explanations are offered in Table~\ref{table:summary_datasets}.

Here we present the results of fingerprint identification presented briefly in~\ref{subsec:performance}. To solve the HE-Cossim methodology's efficiency-performance balance problem, we find the appropriate feature size of the face recognition model, as we demonstrate the performance degradation of the fingerprint recognition task on PolyU datasets. The comparison of Rank-1 accuracies corresponding to each feature size is shown in Figure~\ref{fig:finger_poly_performace_table}. Both experiments on contact-based and contactless datasets do not significantly fail to identify IDs in 1:N recognition with feature size 16. Definitely, the fingerprints are normalized to compare the facial domain, which might explain why the decrease is observed as smaller than Table~\ref{table:face_performance_table} on face datasets.

\begin{figure}[ht]
\centering
    \subfigure[]{
        \includegraphics[width=0.45\linewidth]{figures/Contact PolyU.pdf}
        \label{fig:image1}
    }
    \subfigure[]{
        \includegraphics[width=0.45\linewidth]{figures/Contactless PolyU.pdf}
        \label{fig:image2}
    }
\caption{Comparative experimental results in Fingerprint identification on PolyU Cross Sensor Fingerprint Datasets, respectively on (a) Contact-based dataset and (b) Processed Contactless dataset.} 
\label{fig:finger_poly_performace_table}
\end{figure}

\subsubsection{FVC Dataset}
\label{subsubsec:fvc_dataset}
FVC2000~\cite{maio2000fvc2000}, FVC2002~\cite{maio2002fvc2002}, and FVC2004~\cite{maio2004fvc2004} are widely used fingerprint benchmark datasets. Each database contains four sub-databases: DB1, DB2, DB3, and DB4, and each sub-databases are composed of two types: a, and b. For each DB1, 2, and 3, they collected index finger and middle finger data by various sensors for each sub-database, while the DB4 only contains synthesized fingerprints. Each sub-database consists of 800 fingerprint images from 100 subjects. The size and resolution of each dataset are different. 
Figure~\ref{fig:various_fingerprint_images} shows some samples from FVC datasets. Since the domains of the sub-databases are different from each other, most of the previous research conducted their experiments on a single sub-set. We select FVC2002 DB1 for experiments and further ablation studies in~\ref{subsec:preprocessing_description}.

Moreover, to evaluate \sysname identification performance on a much bigger dataset, we form a combined dataset, considering visual continuances. We could use 770 fingerprint subjects and 6,160 images for further fingerprint experiments with these 7-FVC subsets, as well as conduct preprocessing to remove the characteristic of scanning information of each dataset. In this scenario, to avoid the \sysname learn the reader-specific bias, background noises are removed.

\subsubsection{CASIA Dataset}
\label{subsubsec:casia_dataset}
% \textbf{CASIA Fingerprint Image Dataset Version 5.0 (CASIA-FingerprintV5)}
The CASIA Fingerprint Image Dataset Version 5.0~\cite{CASIA} contains 20,000 fingerprint images of 500 volunteers, a total of 4,000 fingerprint subjects. Eight fingers (Thumb to Ring fingers) are used for each volunteer, and 5 images per finger are scanned with the rolled condition. Each fingerprint image was scammed using a URU4000 fingerprint sensor in a session. All fingerprint images are gray-scale with 328$\times$356 pixel resolution. A sample of this dataset is in the Figure~\ref{fig:various_fingerprint_images}.
Finally, we observed that our \sysname could achieve 1:3,000 recognition with high Rank-1 accuracy at feature size 16 (99.97\%) and 128 (99.87\%).

\subsection{Fingerpirnt Preprocessing Techniques}
\label{subsec:preprocessing_description}

Appropriate preprocessing usually comes first to both authentication and Identification systems in most fingerprint literature. 
Three of the preprocessing that we have done in this research are as follows:
\begin{itemize}
    \item \textbf{Segmenting}. As follows the basic fingerprint preprocessing suggested by~\cite{hong1998fingerprint}, We apply histogram equalization to the input image. Then calculate the level 2 norm of the X-axis and Y-axis Sobel-filtered prints. With threshold k, the high-frequency pattern area only remains, generating a fingerprint mask. 
    \item \textbf{Shifting}. The center of the fingerprint pattern point is easily calculated when it is the masked gray-scale input image. This could be optional.
    \item \textbf{Enhancing}. The enhancing algorithm~\cite{gabor1} results in reconstructed lines without small noises, preserving each ridge valley shape. We recommend downsizing the input image before getting an orientation map and Gabor filtering to save time and resources. Moreover, for the researchers who want to extract enhanced fingerprint images, we highly recommend doing segment images before.
\end{itemize}

\begin{figure}[!ht]
\centerline{\includegraphics[width=0.6\linewidth]{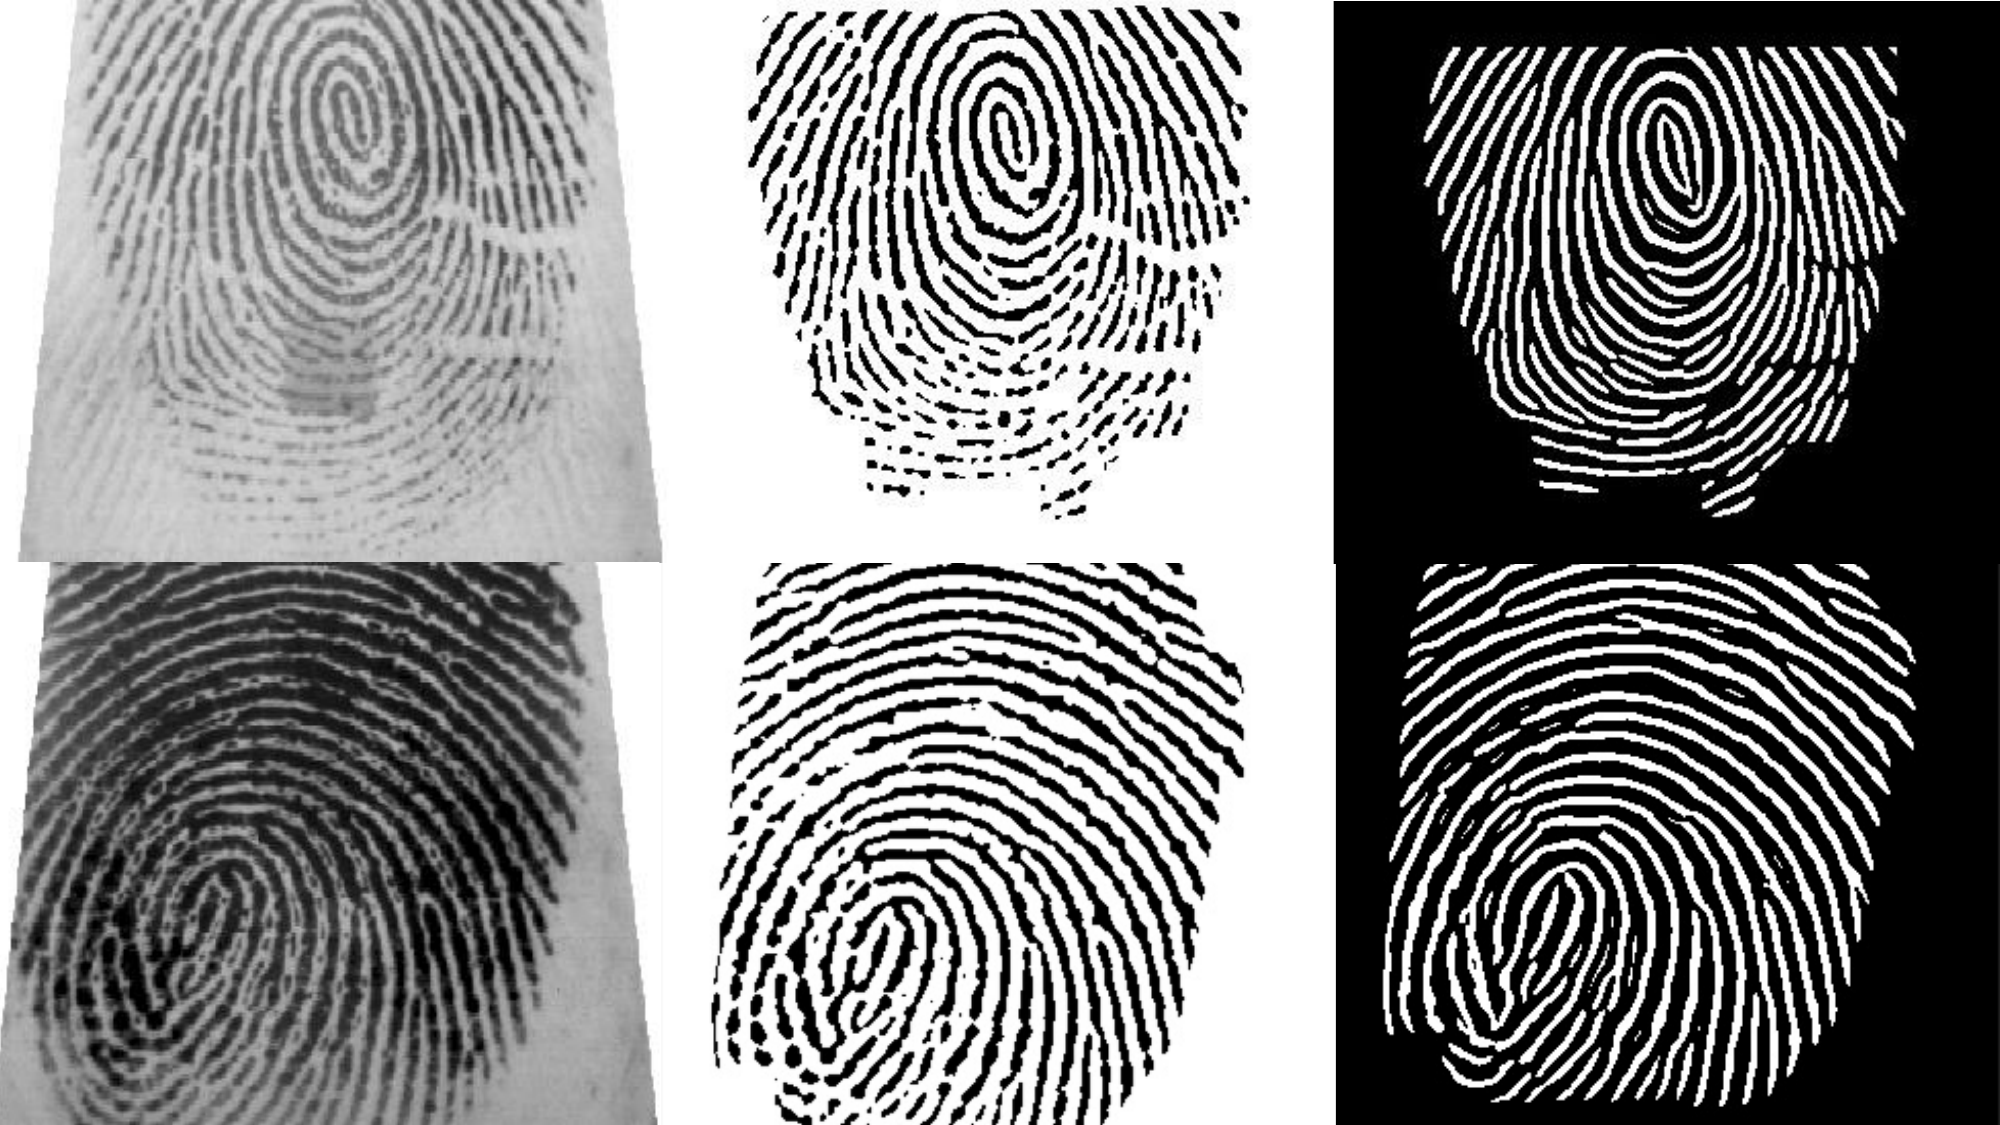}}
\caption{Samples of FVC Datasets preprocessing. From left to right: raw fingerprint, segmented image, and shifted \& enhanced one. }
\label{fig:input_ctxt_structure}
\end{figure}

As several preprocessing improve the low-quality input fingerprint images, we show the ablation study on \sysname 1:N recognition and Blind-touch 1:1 authentication in Section~\ref{subsec:ablation_study}.
Here we report the two results of such ablation experiments in Table~\ref{table:fvc-preprocessing} and~\ref{table:fvc_prerocessing_on_blind_touch}.
Table~\ref{table:fvc_prerocessing_on_blind_touch} shows the effectiveness of the preprocessing methods (Segmenting, Center Shifting) in fingerprint authentication. The experiment is conducted on Blind-Touch with 1:1 authentication. We fixed the threshold as 0.4 in each experiment. 

\begin{table}[ht]
\caption{Effects of preprocessing on fingerprint 1:N identification experiments on newly combined 7-FVC dataset. Rank-1 Accuracy is reported. }
\vspace{0.26cm}
\centering\resizebox{0.5\linewidth}{!}{
\begin{tabular}{c|ccc}
\noalign{\smallskip}\noalign{\smallskip}
\toprule[1.3 pt]
Preprocessing&Not used&Segmenting&Shifting w/ enhancing\\
\hline\hline
Rank-1 (\%)&99.51&99.64&\textbf{99.87}\\
\bottomrule[1.3 pt]
\end{tabular}}
\vspace{-0.2cm}
\label{table:fvc-preprocessing}
\end{table}

\begin{table}[ht]
\caption{Effects of preprocessing in FVC2002 DB1 Dataset on Blind-Touch's 1:1 authentication.}
\vspace{0.26cm}
\setlength{\tabcolsep}{10pt}

\centering\resizebox{0.5\linewidth}{!}{

\begin{tabular}{c| c c c}
\noalign{\smallskip}\noalign{\smallskip}
\toprule[1.3 pt]
 Score \textbackslash Method & Not used & Segmenting & Shifting\\
\hline
\hline
AUC (\%) & 83.03 & 86.50 & \textbf{87.37}  \\
EER (\%) & 20.37  & 13.97 & \textbf{13.64} \\
\bottomrule[1.3 pt]
\end{tabular}}
\vspace{-0.2cm}
\label{table:fvc_prerocessing_on_blind_touch}
\end{table}
% \begin{table}[ht]
% \centering\resizebox{0.9\linewidth}{!}{
% \begin{tabular}{c|c|c|c|c}
% \noalign{\smallskip}\noalign{\smallskip}
% \toprule
% \multicolumn{3}{c|}{Offline Preprocessing}& Spatial&\multirow{2}{*}{\textbf{Acc}} \\ \cline{1-3}
% % \multicolumn{3}{c|}{\textbf{Offline Preprocessing}}&\textbf{ Online Preprocessing} & \multirow{2}{*}{\textbf{Acc}} \\ \cline{1-4}
% Segmenting&Center Shifting&Enhancing&Transformer & \\
% \hline
% \hline
%           &              &            &     & 93.51  \\
% \checkmark&              &            &     & 93.51  \\
% \checkmark&  \checkmark  &            &     & 93.58  \\
% \checkmark&  \checkmark  &\checkmark  &     & 93.73  \\
%           &              &       &\checkmark& 93.92 \\
% \checkmark&              &       &\checkmark& 94.24 \\
% \checkmark& \checkmark   &       &\checkmark& 94.49 \\
% \checkmark&\checkmark &\checkmark&\checkmark&\textbf{94.53} \\
% \bottomrule
% \end{tabular}}
% \caption{Effects of preprocessing on fingerprint identification experiments on FVC2002 DB1. Rank-1 Accuracy is reported. }
% \label{table:fvc-preprocessing}
% \end{table}
